# Supplementary material for: Spectral Statistics of the Sample Covariance Matrix for High Dimensional Linear Gaussians
Source: arXiv:2312.05794 source file (2023-12-10)
Supplement: Supplementary file 1 [file appendix.tex]

\section{Appendix}
\begin{align}
    \langle y_{n-1},\hat{e}_{i+1} \rangle=\lambda \langle y_{n-1},\hat{e}_i \rangle+\langle w_{i},e_{n-1}\rangle+\langle y_{n},\hat{e}_{i}\rangle
\end{align}

\begin{align}
    \nonumber & \langle y_{n-1},y_{n}\rangle= \sum_{i=1}^{N}\bigg(\sum_{t=1}^{i}\lambda^{i-t}\langle w_{t-1},e_{n-1}\rangle + \sum_{t=1}^{i-1} \lambda^{i-t-1} \langle w_{t-1},e_{n}\rangle\bigg)\bigg( \sum_{t=1}^{i} \lambda^{i-t}\langle w_{t-1},e_{n}\rangle  \bigg) \\ \nonumber &= \sum_{i=1}^{N}\bigg( \sum_{t=1}^{i}\lambda^{i-t}\langle w_{t-1},e_{n-1}\rangle \bigg)\bigg( \sum_{t=1}^{i} \lambda^{i-t}\langle w_{t-1},e_{n}\rangle \bigg)+ \sum_{i=1}^{N}\bigg( \sum_{t=1}^{i-1}\lambda^{i-t-1}\langle w_{t-1},e_{n}\rangle \bigg)\bigg( \sum_{t=1}^{i-1} \lambda^{i-t}\langle w_{t-1},e_{n}\rangle+\langle w_{i-1}, e_{n}\rangle \bigg)\\ \nonumber & = \sum_{i=1}^{N}\Bigg[ \sum_{t=1}^{i-1}\lambda^{2(i-t)-1}\langle w_{t-1},e_{n}\rangle^{2}\\ \nonumber &+\bigg( \underbrace{\langle \sum_{t=1}^{i}\lambda^{i-t} w_{t-1},e_{n-1}\rangle}_{\langle s_{i}, e_{n-1}\rangle} \bigg)\bigg( \underbrace{\langle \sum_{t=1}^{i} \lambda^{i-t} w_{t-1},e_{n}\rangle}_{\langle s_{i}, e_{n}\rangle}  \bigg) + \langle w_{i-1}, e_{n}\rangle \sum_{t=1}^{i}\lambda^{i-t}\langle w_{t-1},e_{n-1}\rangle  \Bigg]
\end{align}

 Notice that:
    \begin{align}
    \sum_{j=1}^{n} \frac{1}{\sigma_{j}^{2}(X_{-})} \leq \sqrt{\sum_{j=1}^{n} \frac{n}{\sigma_{j}^{4}(X_{-})}}, \hspace{5pt} \big\|A-\hat{A} \big\|_{F} \leq \sqrt{\sum_{j=1}^{n} \frac{n}{\sigma_{j}^{2}(X_{-})}},      
    \end{align}
    where first inequality follows from Cauchy-Schwarz and second inequality follows from negative second moment estimate. Therefore, 
    \begin{equation}
        \sum_{j=1}^{n} \frac{n}{\sigma_{j}^{2}(X_{-})} \leq \sqrt{\sum_{j=1}^{n} \frac{n^{3}}{\sigma_{j}^{4}(X_{-})}}
    \end{equation}
    and 
    \begin{equation}
        \big\|A-\hat{A} \big\|_{F} \leq  \bigg(\sum_{j=1}^{n} \frac{n\sigma_{1}^{2}(X_{-})}{\sigma_{j}^{4}(X_{-})}\bigg)^{\frac{1}{2}}\land \bigg(\sum_{j=1}^{n} \frac{n^{3}}{\sigma_{j}^{4}(X_{-})}\bigg)^{\frac{1}{4}}.
    \end{equation}
     Now we will try to compute the correlation
    \begin{align}
    \nonumber & \big(\mathbb{E}\langle y_{n-1},y_{n}\rangle\big)^{2}=\lambda^{-4}\sum_{i=1}^{N}\Bigg[ \bigg( \sum_{t=1}^{i-1}\lambda^{4(i-t)} \bigg)^{2}+2\sum_{i'>i}\bigg( \sum_{t=1}^{i-1}\lambda^{4(i-t)}\bigg) \bigg(\sum_{t=1}^{i'-1}\lambda^{4(i'-t)}\bigg)  \Bigg] \\ \nonumber & =\lambda^{-4}\sum_{i=1}^{N}\Bigg[ \bigg( \sum_{t=1}^{i-1}\lambda^{4(i-t)} \bigg)^{2}+2\sum_{i'>i}\bigg( \sum_{t=1}^{i-1}\lambda^{4(i-t)}\bigg) \bigg(\lambda^{4(i'-i)}\sum_{t=1}^{i-1}\lambda^{4(i-t)}+ \sum_{t=i}^{i'-1} \lambda^{4(i'-t)} \bigg)  \Bigg]\\ \nonumber & = \lambda^{-4}\sum_{i=1}^{N}\Bigg[ \bigg( \sum_{t=1}^{i-1}\lambda^{4(i-t)} \bigg)^{2}+2\bigg( \sum_{t=1}^{i-1}\lambda^{4(i-t)}\bigg)^{2}\sum_{i'>i}\lambda^{4(i'-i)} + 2\bigg( \sum_{t=1}^{i-1}\lambda^{4(i-t)}\bigg)\sum_{i'>i}\sum_{t=i}^{i'-1} \lambda^{4(i'-t)} \bigg)  \Bigg]\\ \nonumber &  = \lambda^{-4} \sum_{i=1}^{N}\bigg( \sum_{t=1}^{i-1}\lambda^{4(i-t)} \bigg)^{2}\bigg(1+2\sum_{i'>i}\lambda^{4(i'-i)}\bigg)+2 \lambda^{-4}\sum_{i=1}^{N}\sum_{t=1}^{i-1} \lambda^{4(i-t)} \sum_{i'>i} \sum_{t'=i}^{i'-1}\lambda^{4(i'-t')}= \\ \nonumber &  \lambda^{-4} \sum_{i=1}^{N}\bigg( \sum_{t=1}^{i-1}\lambda^{4(i-t)} \bigg)^{2}\bigg(1+2\sum_{i'>i}\lambda^{4(i'-i)}\bigg)+2 \lambda^{-4}\sum_{i=1}^{N}\sum_{t=1}^{i-1}\sum_{i'>i} \sum_{\hspace{10pt}t'>i-1}^{i'-1}\lambda^{4(i'-t')}\lambda^{4(i-t)}=\\ \nonumber &\lambda^{-4} \sum_{i=1}^{N}\bigg( \sum_{t=1}^{i-1}\lambda^{8(i-t)}+2\lambda^{4(i-t)}\sum_{t'>t} \lambda^{4(i-t')} \bigg)\bigg(1+2\sum_{i'>i}\lambda^{4(i'-i)}\bigg)+2 \lambda^{-4}\sum_{i=1}^{N}\sum_{t=1}^{i-1}\sum_{i'>i} \sum_{\hspace{10pt}t'>i-1}^{i'-1}\lambda^{4(i'-t')}\lambda^{4(i-t)}\\  \nonumber & =2\lambda^{-4}\sum_{i=1}^{N}\sum_{t=1}^{i-1}\lambda^{8(i-t)} \sum_{i'>i} \lambda^{4(i'-i)}+\lambda^{-4}\sum_{i=1}^{N}\sum_{t=1}^{i-1}\lambda^{8(i-t)}+2\lambda^{-4}\sum_{i=1}^{N}\sum_{t=1}^{i-1}\lambda^{4(i-t)} \sum_{t'>t} \lambda^{4(i'-t)}\\ \nonumber & +4\lambda^{-4}\sum_{i=1}^{N}\sum_{t=1}^{i-1}\lambda^{4(i-t)} \sum_{t'>t} \lambda^{4(i'-t)}\sum_{i'>i} \lambda^{4(i'-i)}+2 \lambda^{-4}\sum_{i=1}^{N}\sum_{t=1}^{i-1}\sum_{i'>i} \sum_{\hspace{10pt}t'>i-1}^{i'-1}\lambda^{4(i'-t')}\lambda^{4(i-t)} \end{align}

\begin{flalign}
\nonumber [X_{-}]_{k,n}&= \sum_{m=0}^{ n-k } \binom{n-1}{m} \lambda^{n-1-m} \langle w_{0} ,e_{m+k}  \rangle+\binom{n-2}{m} \lambda^{n-2-m} \langle w_{1} ,e_{m+k}  \rangle+  \binom{n-3}{m} \lambda^{n-3-m} \langle w_{1} ,e_{m+k}  \rangle+\ldots \\ & \nonumber  + \sum_{m=0}^{n-(k+1)} \binom{n-(k+1)}{m} \lambda^{n-(k+1)-m}\langle w_{k} ,e_{m+k}  \rangle  + \ldots+ \sum_{m=0}^{1} \binom{1}{m} \lambda^{1-m} \langle w_{n-2} ,e_{m+k} \rangle + \langle w_{n-1}, e_{k} \rangle
\end{flalign}
\begin{align}
& \label{eq:causalrowdep}
    [X_{-}]_{k,i}= \sum_{t=1}^{i} \sum_{m=0}^{(i-t) \land (n-k) } \binom{i-t}{m} \lambda^{i-t-m} \big\langle w_{t-1} ,e_{m+k} \big \rangle
\end{align}
Now for $j,k \in [n]$
\begin{align}
 \nonumber [X_{-}E^{*}]_{j,k}&=\sum_{i=1}^{N} [X_{-}]_{j,i} \langle w_{i-1},e_{k}\rangle=\sum_{i=1}^{N}\sum_{t=1}^{i} \sum_{m=0}^{(i-t) \land (n-j) } \binom{i-t}{m} \lambda^{i-t-m} \big\langle w_{t-1} ,e_{m+j} \big \rangle  \langle w_{i-1},e_{k}\rangle \\& \nonumber = \sum_{i=1}^{N}  \langle w_{i-1},e_{k}\rangle  \langle w_{i-1},e_{j}\rangle +\langle w_{i-1},e_{k}\rangle \sum_{t=1}^{i-1} \sum_{m=0}^{(i-t) \land (n-j) } \binom{i-t}{m} \lambda^{i-t-m} \big\langle w_{t-1} ,e_{m+j} \big \rangle \hspace{5pt} \textit{therefore,} 
\end{align}
\begin{align}
   \nonumber \sum_{j,k}|[X_{-}E*]_{j,k}|^{2}&=\sum_{j,k} \sum_{i=1}^{N}\bigg( \langle w_{i-1},e_{k}\rangle  \langle w_{i-1},e_{j}\rangle +\langle w_{i-1},e_{k}\rangle \sum_{t=1}^{i-1} \sum_{m=0}^{(i-t) \land (n-j) } \binom{i-t}{m} \lambda^{i-t-m} \big\langle w_{t-1} ,e_{m+j} \big \rangle \bigg) \\ & \nonumber \times \Bigg[\bigg( \langle w_{i-1},e_{k}\rangle  \langle w_{i-1},e_{j}\rangle +\langle w_{i-1},e_{k}\rangle \sum_{t=1}^{i-1} \sum_{m=0}^{(i-t) \land (n-j) } \binom{i-t}{m} \lambda^{i-t-m} \big\langle w_{t-1} ,e_{m+j} \big \rangle \bigg) \\ & \nonumber \hspace{15pt}+2\sum_{i'>i}^{N}\bigg( \langle w_{i'-1},e_{k}\rangle  \langle w_{i'-1},e_{j}\rangle +\langle w_{i'-1},e_{k}\rangle \sum_{t=1}^{i'-1} \sum_{m=0}^{(i'-t) \land (n-j) } \binom{i-t}{m} \lambda^{i'-t-m} \big\langle w_{t-1} ,e_{m+j} \big \rangle \bigg)\Bigg] \\ & \nonumber \hspace{10pt}:=\big\|X_{-}E^{*}\big\|_{F}^{2}
\end{align}
Compare with:
\begin{equation}
\|X_{-}\|_{F}^{2}:=\sum_{i=1}^{N} \sum_{j=1}^{n} \sum_{s,t=1}^{i} \sum_{m=0}^{(i-t)\land (n-j)} \sum_{m'=0}^{(i-s)\land (n-j)}  \binom{i-t}{m} \binom{i-s}{m'} \lambda^{i-t-m} \overline{\lambda^{i-s-m'}} \langle w_{t-1},e_{j+m}\rangle \overline{\langle w_{s-1},e_{j+m'}\rangle}
\end{equation}

\paragraph{Spectrum of the precision matrix}
\begin{align}
    \|(X_{-}X_{-})^{-1}\|_{F}=\sqrt{Tr\big((X_{-}X_{-}^{*})^{-2}\big)}=\sqrt{\sum_{j=1}^{n}d_{j}^{-4}+2\sum_{k>j}|v_{j,k}|^{2} }
\end{align}
 As we will see shortly afterwards, elementwise estimation error is an inner product between the rows of the Gaussian ensemble and and columns of the pseudo-inverse, it will be helpful to translate preceding constraints into constraints on columns of pseudo-inverse.     
\begin{corollary}
\label{cor:c_kd}
    [Exact Error in Frobenius norm] Let $\hat{e}_{i}$ be the canonical basis of $\mathbb{C}^{N}$
\begin{align}
    \|A-\hat{A}\|_{F}=\sqrt{\sum_{j,k=1}^{n} \bigg|\sum_{i=1}^{N} \langle w_{i},e_{j}\rangle \langle c_{k},\hat{e}_{i}\rangle \bigg|^{2}},
\end{align}
    where for each $k \in [1,2,\ldots,n]$, $c_{k} \in \mathbb{C}^{N}, \|c_{k}\|^{2}= \frac{1}{d^{2}(y_k,n_k)}$ and satisfies:
\begin{equation}
\label{eq:normaleq}
    \sum_{i=1}^{N} \bigg[ \sum_{t=1}^{i} \langle A^{i-t}w_{t-1},e_{j}\rangle  \bigg]\langle c_{k}, \hat{e}_{i}\rangle= \delta_{j}(k),
\end{equation}
for every $j \in [1,2,\ldots,n]$ 
\end{corollary}
\begin{proof}
    Consider the pseudo-inverse
    \[X_{-}^{*} (X_{-}X_{-}^{*})^{-1} =
\begin{bmatrix}
    \vert & \vert & \vert & \vert &\vert \\
    \vert & \vert & \vert & \vert &\vert \\
    c_{1} & c_{2} & \vert & c_{n-1} &c_{n}   \\
    \vert & \vert & \vert & \vert &\vert \\
    \vert & \vert & \vert & \vert &\vert
\end{bmatrix}
\]
as inner product of $X_{-}^{*} \big(X_{-}X_{-}^{*}\big)^{-1}e_{j}$ with $X_{-}^{*}e_{k}=:y_{k}$ for $k \neq j$ is zero; so for each $j \in [n]$ , $c_{j}:=X_{-}^{*} \big(X_{-}X_{-}^{*}\big)^{-1}e_{j}$ is orthogonal to $n_{j}$
\begin{align}
    & \nonumber \sum_{i=1}^{N} [X_{-}]_{j,i} \langle c_{k}, \hat{e}_{i}\rangle= \delta_{j}(k), \hspace{10pt} \textit{implies} \hspace{10pt}  \sum_{i=1}^{N} \bigg[ \sum_{t=1}^{i} \langle A^{i-t}w_{t-1},e_{j}\rangle  \bigg]\langle c_{k}, \hat{e}_{i}\rangle= \delta_{j}(k),
\end{align}
Also notice that $c_{k}:=X_{-}^{*}(X_{-}X_{-}^{*})^{-1}e_{k}$ and
\begin{equation}
    \big\|c_{k}\|^{2} =\big\langle X_{-}^{*}(X_{-}X_{-}^{*})^{-1}e_{k},X_{-}^{*}(X_{-}X_{-}^{*})^{-1}e_{k}\rangle=\frac{1}{d^{2}(y_k,n_k)}.
\end{equation}
\end{proof}
\begin{theorem}
    \begin{align}
        \nonumber & \mathbb{E}\langle y_{n-1},y_{n}\rangle \langle y_{n-1},y_{n}\rangle -\big( \mathbb{E}\langle y_{n-1},y_{n}\rangle \big)^{2}=2\sum_{i=1}^{N-1}\sum_{i'>i}\lambda^{2(i'-i)} \bigg(\sum_{t=1}^{i}\lambda^{2(i-t)}\bigg)^{2}\\ \nonumber & + 3\lambda^{-4}\sum_{t=1}^{N-1} \bigg( \sum_{l=1}^{N-t} \lambda^{2l}  \bigg)^{2}+ 2\lambda^{-4}\sum_{t=1}^{N-1}\sum_{t'>t}^{N-1} \sum_{l=1}^{N-t}   \sum_{l'=1}^{N-t'} \lambda^{2(l'+l)} + \sum_{i=1}^{N-1}\sum_{t=1}^{i} \lambda^{2(i-t)} \\ \nonumber &-\\ \nonumber & =\sum_{i=1}^{N}\Bigg[2\sum_{i'>i}\lambda^{2(i'-i)} \bigg(\sum_{t=1}^{i}\lambda^{2(i-t)}\bigg)^{2}- 2\lambda^{-4}\bigg(\sum_{t=1}^{i-1}\lambda^{4(i-t)} \bigg)^{2}\sum_{i'>i}\lambda^{4(i'-i)}-\lambda^{-4}\bigg(\sum_{t=1}^{i-1}\lambda^{4(i-t)} \bigg)^{2} \Bigg]\\ \nonumber &+  2\lambda^{-4}\sum_{t=1}^{N-1}\sum_{t'>t}^{N-1} \sum_{l=1}^{N-t}   \sum_{l'=1}^{N-t'} \lambda^{2(l'+l)}-2 \lambda^{-4}\sum_{i=1}^{N}\sum_{t=1}^{i-1}  \sum_{i'>i} \sum_{t'=i}^{i'-1}\lambda^{4(i-t)}\lambda^{4(i'-t')}\\ \nonumber&+3\lambda^{-4}\sum_{t=1}^{N-1} \bigg( \sum_{l=1}^{N-t} \lambda^{2l}  \bigg)^{2}+\sum_{i=1}^{N}\sum_{t=1}^{i} \lambda^{2(i-t)}  
    \end{align}
\end{theorem}
So let us compute the size of $\|y_2\|$
\begin{align}
    \nonumber [X_{-}]_{2,(n-1)}& =\sum_{t=1}^{(n-1)} \sum_{m=0}^{(n-1-t)} \binom{n-1-t}{m}\lambda^{n-1-t-m} \langle w_{t-1} , e_{m+2} \rangle=\sum_{m=0}^{n-2} \binom{n-2}{m} \lambda^{n-2-m} \langle w_{0} , e_{m+2} \rangle \\ & \nonumber + \sum_{m=0}^{n-3} \binom{n-3}{m} \lambda^{n-3-m} \langle w_{1} , e_{m+2} \rangle+ \ldots + \sum_{m=0}^{1} \binom{1}{m} \lambda^{1-m} \langle w_{n-3},e_{m+2} \rangle+ \langle w_{n-2},e_{2}\rangle
    \end{align}
    \begin{align}
    \nonumber Var([X_{-}]_{2,n-1})&=\sum_{k=2}^{n}\sum_{m=0}^{n-k} \binom{n-k}{m}^{2} \lambda^{2(n-k-m)}\geq \lambda^{2n}\sum_{k=2}^{n} \frac{1}{\lambda^{2k}}\binom{2(n-k)}{n-k} \geq \lambda^{2n}4^{n} \underbrace{\sum_{k=2}^{n} 
    \frac{1}{4^{k} \lambda^{2k}\sqrt{\pi(n-k+\frac{1}{3})}}}_{S_{\lambda,n}(2)}
\end{align}
\begin{align}
& \nonumber \sum_{k=1}^{n} \lambda^{2(n-k)} \sum_{m=0}^{n-k} \binom{n-k}{m}^{2} \lambda^{-2m} \geq \sum_{k=1}^{n} \lambda^{2(n-k)} \sum_{m=0}^{n-k} \binom{n-k}{m}^{2}=\sum_{k=1}^{n} \lambda^{2(n-k)} \binom{2(n-k)}{n-k}  \\ & \label{eq:ldghf} \geq \sum_{k=1}^{n} \lambda^{2(n-k)} \frac{4^{(n-k)}}{\sqrt{\pi(n-k+\frac{1}{3})}}=,  
\end{align}
Now notice that $S_{\lambda,n}(1)-S_{\lambda,n}(2)=\frac{1}{4\lambda^{2} \sqrt{\pi(n-1+\frac{1}{3})}}$
paragraph{Controlling the trace of Sample Covariance matrix}
Now we actually compute $\big\| X_{-}E^{*}\big\|_{F}$, recall that:
\begin{equation}
 [X_{-}]_{j,i}= \sum_{t=1}^{i} \sum_{m=0}^{(i-t) \land (n-j) } \binom{i-t}{m} \lambda^{i-t-m} \big\langle w_{t-1} ,e_{m+j} \big \rangle.   
\end{equation}
So let us compute the size of $\|y_2\|$
\begin{align}
    & \nonumber [X_{-}]_{2,(n-1)}=\sum_{t=1}^{(n-1)} \sum_{m=0}^{(n-1-t)} \binom{n-1-t}{m}\lambda^{n-1-t-m} \langle w_{t-1} , e_{m+2} \rangle=\sum_{m=0}^{n-2} \binom{n-2}{m} \lambda^{n-2-m} \langle w_{0} , e_{m+2} \rangle \\ & \nonumber + \sum_{m=0}^{n-3} \binom{n-3}{m} \lambda^{n-3-m} \langle w_{0} , e_{m+3} \rangle+ \ldots + \sum_{m=0}^{1} \binom{1}{m} \lambda^{1-m} \langle w_{n-3},e_{m+2} \rangle+ \langle w_{n-2},e_{2}\rangle \\ & \nonumber Var([X_{-}]_{2,n-1})=\sum_{k=2}^{n}\sum_{m=0}^{n-k} \binom{n-k}{m}^{2} \lambda^{2(n-k-m)}=\sum_{k=2}^{n}\lambda^{2(n-k)}\binom{2(n-k)}{n-k} \\ & \nonumber \geq \lambda^{2n}4^{n} \underbrace{\sum_{k=2}^{n} 
    \frac{1}{4^{k} \lambda^{2k}\sqrt{\pi(n-k+\frac{1}{3})}}}_{S_{\lambda,n}(2)}
\end{align}
what is the the typical size of this thing 
Consider data matrix populated by $n-$ dimensional S-w-SSCs with stable mode $\lambda \in (0,1)$. When time index $i=n$, with some extra effort one can show that first row of the $n-$ th column of data matrix is a weighted sum of $\frac{n}{2}(n-1)$ stanadard normals, mathematically:
\begin{align}
       \nonumber [X_{-}]_{1,n}&=\sum_{m=0}^{n-1 } \binom{n-1}{m} \lambda^{n-1-m} \big \langle w_{0}, e_{m+1} \big \rangle  \nonumber +\sum_{m=0}^{n-2} \binom{n-2}{m} \lambda^{n-2-m} \big \langle w_{1},e_{m+1} \big \rangle+\ldots \\ & \nonumber   + \sum_{m=0}^{1} \binom{1}{m} \lambda^{1-m}  \big \langle w_{n-2}, e_{m+1} \big \rangle + \big \langle w_{n-1}, e_{1} \big \rangle, \hspace{5pt} \textit{and} 
\end{align}
\begin{equation}
    Var([X_{-}]_{1,n})=\sum_{k=1}^{n}\sum_{m=0}^{n-k} \binom{n-k}{m}^{2} \lambda^{2(n-k-m)}
\end{equation}
 Let $\lambda \in (0,1)$ implying that $[X_{-}]_{1,n}$ is normally distributed with variance:
\begin{align}
& \nonumber \sum_{k=1}^{n} \lambda^{2(n-k)} \sum_{m=0}^{n-k} \binom{n-k}{m}^{2} \lambda^{-2m} \geq \sum_{k=1}^{n} \lambda^{2(n-k)} \sum_{m=0}^{n-k} \binom{n-k}{m}^{2}=\sum_{k=1}^{n} \lambda^{2(n-k)} \binom{2(n-k)}{n-k}  \\ & \label{eq:ldghf} \geq \sum_{k=1}^{n} \lambda^{2(n-k)} \frac{4^{(n-k)}}{\sqrt{\pi(n-k+\frac{1}{3})}}=4^{n} \lambda^{2n} \underbrace{\sum_{k=1}^{n} \frac{1}{4^{k}\lambda^{2k} \sqrt{\pi(n-l+\frac{1}{3})}}}_{:=S_{\lambda,n}(1)},  
\end{align}
Now notice that $S_{\lambda,n}(1)-S_{\lambda,n}(2)=\frac{1}{4\lambda^{2} \sqrt{\pi(n-1+\frac{1}{3})}}$

\begin{theorem}
Overall variance $Var([X_{-}]_{1,n})+ Var([X_{-}]_{2,n-1})+\ldots + Var([X_{-}]_{n-1,2})+Var([X_{-}]_{n,1})$ is:
\begin{align}
    \\ & \nonumber \lambda^{2(n-1)}\sum_{m=0}^{n-1} \binom{n-1}{m}^{2} \lambda^{-2m}+2\lambda^{2(n-2)}\sum_{m=0}^{n-2} \binom{n-2}{m}^{2} \lambda^{-2m}+3\lambda^{2(n-3)}\sum_{m=0}^{n-3} \binom{n-3}{m}^{2} \lambda^{-2m} +\ldots + n \\ & \nonumber \geq \sum_{k=1}^{n}k \lambda^{2(n-k)}\sum_{m=0}^{n-k} \binom{n-k}{m}^{2}=\sum_{k=1}^{n} k\lambda^{2(n-k)} \binom{2(n-k)}{n-k} \geq \sum_{k=1}^{n} k\lambda^{2(n-k)} \frac{4^{(n-k)}}{\sqrt{\pi(n-k+\frac{1}{3})}}\\ & \nonumber=4^{n}\lambda^{2n} \sum_{k=1}^{n} \frac{k \lambda^{-2k}}{4^{k}\sqrt{\pi(n-k+\frac{1}{3})}}  
\end{align}
Therefore, for all $k \in [n]$
\begin{equation}
    Var\big([X_{-}]_{n-k+1,k}\big) \geq 4^{n}\lambda^{2n}S_{\lambda,n}(n-k+1)
\end{equation}
\end{theorem}
\paragraph{Off-diagonal entries of sample covariance matrix + correlations}

\begin{equation}
 \langle y_{j}, \hat{e}_{i} \rangle= \sum_{t=1}^{i} \sum_{m=0}^{(i-t) \land (n-j) } \binom{i-t}{m} \lambda^{i-t-m} \big\langle w_{t-1} ,e_{m+j} \big \rangle.   
\end{equation}
For example we will neeed to compute $\langle y_j,y_{j+1} \rangle$.Now define the correlation function between first column-last row of the data matrix $\langle y_{n},\hat{e}_{1}\rangle$, and $\langle y_1 , \hat{e}_{n}\rangle$ as:
\begin{align}
    C_{[(n,1),(1,n)]}:=\frac{\mathbb{E}[\langle y_{n},\hat{e}_{1}\rangle \langle y_1 , \hat{e}_{n}\rangle]} {\sqrt{Var(\langle y_{n},\hat{e}_{1}\rangle)}\sqrt{Var(\langle y_1 , \hat{e}_{n}\rangle)}}=\bigg(\sum_{k=1}^{n}\sum_{m=0}^{n-k} \binom{n-k}{m}^{2} \lambda^{2(n-k-m)}\bigg)^{-\frac{1}{2}}
\end{align}
\subsection{Various error statistics}

\begin{align}
     & \nonumber \big\|A-\hat{A} \big\|_{F}= \big\|EX_{-}^{*}(X_{-}X_{-}^{*})^{-1} \big\|_{F}=\sqrt{Tr\big(EX_{-}^{*}(X_{-}X_{-}^{*})^{-2}X_{-}E^{*}\big)} =\sqrt{Tr\big(X_{-}E^{*}EX_{-}^{*}(X_{-}X_{-}^{*})^{-2}\big)} \\ & \nonumber= \sqrt{Tr\big((X_{-}X_{-}^{*})^{-1}X_{-}E^{*}EX_{-}^{*}(X_{-}X_{-}^{*})^{-1}\big)}:= \big\| (X_{-}X_{-}^{*})^{-1}X_{-}E^{*} \big\|_{F}=\sqrt{\sum_{k=1}^{n} \sigma_{k}^{2} \bigg( (X_{-}X_{-}^{*})^{-1}X_{-}E^{*} \bigg)}\\ 
\end{align}   
\begin{equation}
    \sigma_{k} \bigg( (X_{-}X_{-}^{*})^{-1}X_{-}E^{*} \bigg):= \max_{V \subset \mathbb{R}^{n}: dim(V)=k.} \hspace{5pt} \min_{a \in S^{n-1} \cap V} \big\| (X_{-}X_{-}^{*})^{-1}X_{-}E^{*}a \big\|
\end{equation}
Now notice that
\begin{align}
    & \nonumber \frac{\big\|X_{-}E^{*}a\big\|}{\sigma_{1}\big(X_{-}X_{-}^{*} \big)}=\sigma_{n}\bigg(\big(X_{-}X_{-}^{*})^{-1}\bigg) \big\|X_{-}E^{*}a\big\| \leq \big\| (X_{-}X_{-}^{*})^{-1}X_{-}E^{*}a \big\| \\ & \nonumber \leq \sigma_{1}\bigg((X_{-}X_{-}^{*})^{-1}\bigg) \big\|X_{-}E^{*}a\big\|=\frac{\big\|X_{-}E^{*}a\big\|}{\sigma_{n}\big(X_{-}X_{-}^{*} \big)}
\end{align}
Now recall that:
\begin{equation}
\sigma_{1}\big(X_{-}X_{-}^{*}\big)=\sqrt{\lambda_{max} \big( (X_{-}X_{-}^{*})^{2}\big)}=\sqrt{\lambda_{max}^{2} (X_{-}X_{-}^{*})}=\lambda_{max}(X_{-}X_{-}^{*})=:\sigma_{1}^{2}(X_{-})
\end{equation}
Similarly $\sigma_{n}(X_{-}X_{-}^{*})=\sigma_{n}^2(X_{-})$ and:
\begin{equation}
    \frac{\big\|X_{-}E^{*}a\big\|}{\sigma_{1}^{2}(X_{-})} \leq \big\| (X_{-}X_{-}^{*})^{-1}X_{-}E^{*}a \big\| \leq \frac{\big\|X_{-}E^{*}a\big\|}{\sigma_{n}^{2}(X_{-})}.
\end{equation}
Which now allows us to instead write 
\begin{equation}
    \frac{\sigma_{k}(X_{-}E^{*})}{\sigma_{1}^{2}(X_{-})} \leq  \sigma_{k}\bigg( (X_{-}X_{-}^{*})^{-1}X_{-}E^{*} \bigg) \leq \frac{\sigma_{k}(X_{-}E^{*})}{\sigma_{n}^{2}(X_{-})}
\end{equation}

we find it easier to consider a somewhat similar error formulation
\begin{align}
    \label{eq:srkfill} \frac{\big\| EX_{-}^{*}\big\|_{F}}{\sigma_{1}^{2}(X_{-})} \leq \big\|A- \hat{A}\big\|_{F} \leq \frac{\big\| EX_{-}^{*}\big\|_{F}}{\sigma_{n}^{2}(X_{-})},
\end{align}
to show that for high dimensional spatially inseparable dynamics OLS error stays bounded away from zero.
\begin{remark}
    But this will have a huge gap when order of the smallest and largest singular values is different. So instead we will now try
\end{remark}
\begin{align}
    & \nonumber \sigma_{n}(EX_{-}^{*})\big\|(X_{-}X_{-}^{*})^{-1}\big\|_{F} \leq \big\|A-\hat{A} \big\|_{F} \leq \sigma_{1}(EX_{-}^{*}) \big\|(X_{-}X_{-}^{*})^{-1}\big\|_{F} \\ & \nonumber \sigma_{n}(EX_{-}^{*}) \bigg(\sum_{j=1}^{n} \sigma_{j}^{-4}(X_{-})\bigg)^{\frac{1}{2}} \leq \big\|A-\hat{A} \big\|_{F} \leq \sigma_{1}(EX_{-}^{*}) \bigg(\sum_{j=1}^{n} \sigma_{j}^{-4}(X_{-})\bigg)^{\frac{1}{2}},
\end{align}
where recall that $\sigma_{j}^{4}(X_{-})=\lambda_{j}^{2}(X_{-}X_{-}^{*})$, eigenvalue of the sample covariance matrix.
In the case of S-w-SSCs we know the correct order of $\|X_{-}\|=\sqrt{N-n+1}e^{\frac{\alpha_{\lambda}n}{2}}$. We can now leverage upon the moment method to conclude:
\begin{equation}
\sum_{k=1}^{n} \sigma_{k}^{2n}(X_{-})=(N-n+1)^{n}e^{\alpha_{\lambda}\frac{n^2}{2}} 
\end{equation}
\begin{theorem}
    [Cauchy's interlacing theorem] 
    \begin{align}
         \nonumber & \bigg(\frac{N}{n-i+1}\bigg)4^{(n-i+1)}\lambda^{2(n-i+1)} \leq \sigma_{i}^{2}(X_{-}) \leq (N-[n-i+1]+1)4^{(n-i+1)}\lambda^{2(n-i+1)} 
    \end{align}
\end{theorem}    
\begin{align}
    \sqrt{ \sum_{i=1}^{n}(n-i+1)^{2} (4\lambda^{2})^{2i}}= (2\lambda)^{4n} \sqrt{\sum_{i=0}^{n-1} \bigg(\frac{i+1}{2^{2i}\lambda^{2i}}\bigg)^{2} }
\end{align}

\begin{theorem}
    \begin{align}
        \nonumber  \big\|A-\hat{A}_{N} \big\|_{F}&= \bigg( \frac{n}{N}\bigg)^{\frac{1}{2}} \bigg( \frac{N-n+1}{N}\bigg)^{\frac{1}{2}}\frac{(2\lambda)^{4n}}{(2\lambda)^{n+2}} \sqrt{\sum_{i=0}^{n-1} \bigg(\frac{i+1}{2^{2i}\lambda^{2i}}\bigg)^{2}} \\ \nonumber &=\bigg( \frac{n}{N}\bigg)^{\frac{1}{2}} \bigg( \frac{N-n+1}{N}\bigg)^{\frac{1}{2}}(2\lambda)^{3n-2} \sqrt{ \sum_{i=0}^{n-1} \bigg(\frac{i+1}{[2\lambda]^{2i}}\bigg)^{2}}
    \end{align}
\end{theorem}
 \begin{proof}    
    \begin{align}
        \nonumber  \big\|A-\hat{A}_{N} \big\|_{F}^{2} & \leq n(N-n+1)4^{n}\lambda^{2n} \bigg(\frac{1}{\sigma_{1}^{4}(X_{-})}+ \frac{1}{\sigma_{2}^{4}(X_{-})}+ \frac{1}{\sigma_{3}^{4}(X_{-})}+\ldots+ {\frac{1}{\sigma_{n}^{4}(X_{-})}} \bigg) \\ \nonumber & \leq 
        \frac{n(N-n+1)}{N^{2}4^{n}4^{2}\lambda^{2n}\lambda^{4}}\sum_{i=1}^{n} (n-i+1)^{2} 4^{2i} \lambda^{4i}
    \end{align}
\end{proof}
\begin{theorem}
\begin{align}
   \bigg(\frac{1}{2\lambda}\bigg)\bigg(\frac{1}{4^{n}\lambda^{2n}n}\bigg)^{\frac{1}{2}}\sqrt{\sum_{i=1}^{n}\frac{4^{i}\lambda^{2i}}{(N-n+i)} }  \leq \|A-\hat{A}_{N}\|_{F} \leq \bigg(\frac{n}{N4^{n+1}\lambda^{2(n+1)}}\bigg)^{\frac{1}{2}}\sqrt{\sum_{i=1}^{n} 4^{i}\lambda^{2i}(n-i+1)}
\end{align}    
\end{theorem}
\begin{figure} [!t]

\begin{center}
\includegraphics[width=0.70\textwidth]{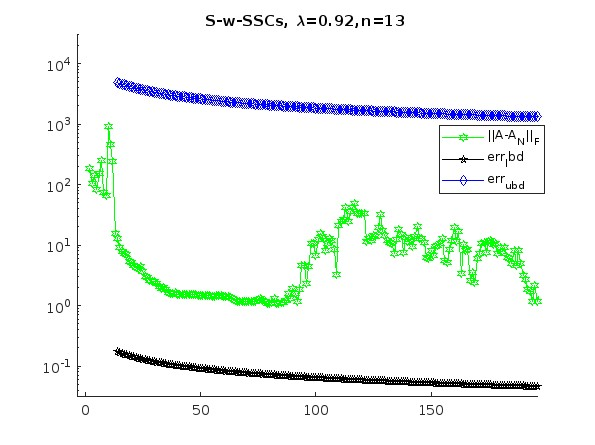}     
\caption{Actual error compared with given upper and lower bounds}  
\label{fig:coverror92sw}
\end{center}                
\end{figure}
It remains only to control:
\begin{align}
    \sum_{i=0}^{n-1} \bigg(\frac{i+1}{2^{2i}\lambda^{2i}}\bigg)^{2}=\sum_{i=0}^{n-1} \bigg(\frac{i+1}{4^{i}\lambda^{2i}}\bigg)^{2}=\sum_{i=0}^{n-1} \bigg(\frac{i+1}{[2\lambda]^{2i}}\bigg)^{2}
\end{align}    
\begin{figure} [!t]
\begin{center}
\includegraphics[width=0.70\textwidth]{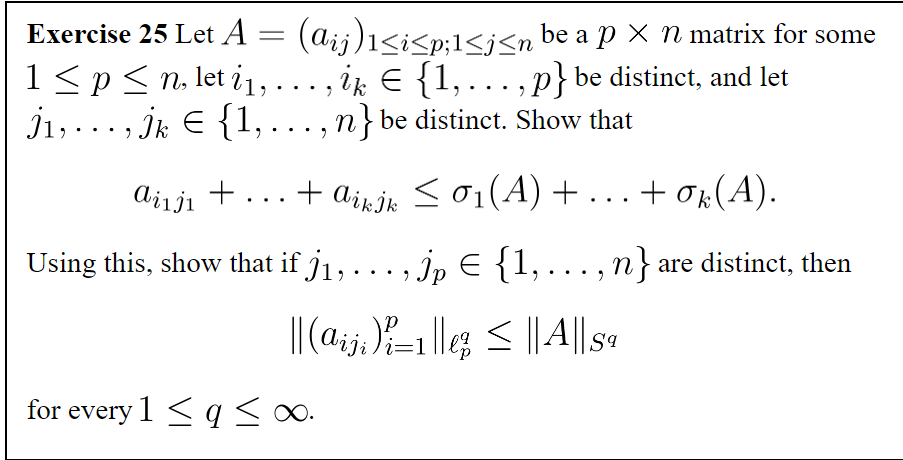}     
\caption{Vareig1} 
\label{fig:vareig1}
\end{center}                
\end{figure}

\begin{figure} [!t]
\begin{center}
\includegraphics[width=0.70\textwidth]{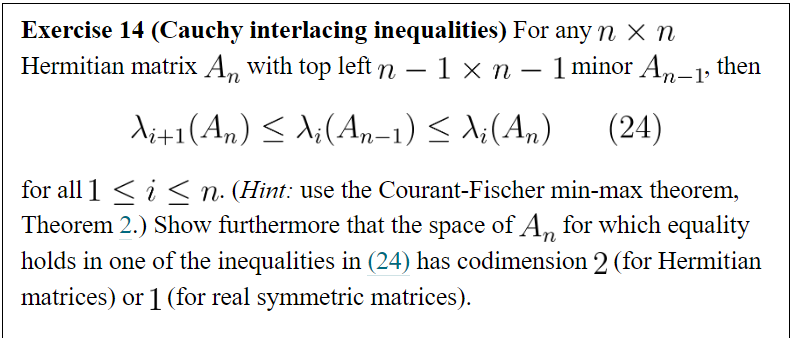}     
\caption{Vareig2} 
\label{fig:vareig2}
\end{center}                
\end{figure}

\begin{figure} [!t]
\begin{center}
\includegraphics[width=0.70\textwidth]{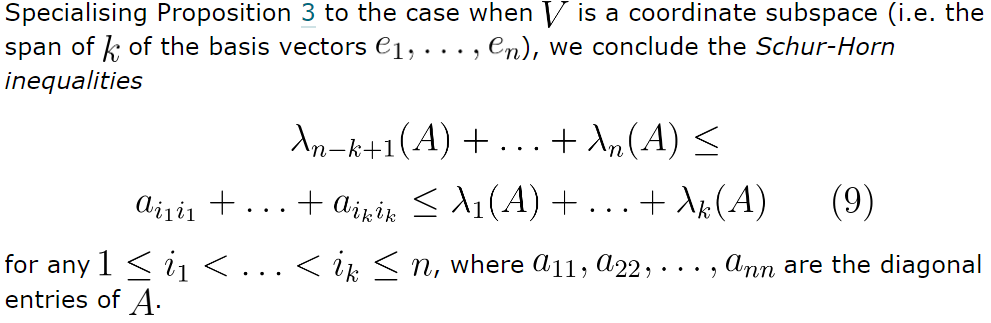}     
\caption{Vareig3} 
\label{fig:vareig3}
\end{center}                
\end{figure}
\section{Self-Normalized Martingale}
If $Im(X_{-})=\mathbb{R}^{n}$, then there exists unitary $[u_{i}]_{i=1}^{n}$ such that
\begin{equation}
    X_{-}X_{-}^{*}u_{i}=\sigma_{i}^{2}(X_{-})u_i.
\end{equation}
Let $v_{i}:=\frac{X_{-}^{*}u_i}{\sigma_{i}}$ which is again unitary and $U:=[u_1, \ldots, u_n] \in \mathbb{R}^{n \times n}$, $V:=[v_1, \ldots, v_{n}] \in \mathbb{R}^{N \times n}$. Now notice that as $U^{*}U=I$, $U^{*}=U^{-1}$ and we can write
\begin{align}
    \nonumber & X_{-}=U \Sigma V^{*}, \hspace{3pt} \big(X_{-}X_{-}^{*}\big)^{-1}=U\Sigma^{-2}U^{*}, \hspace{3pt} \textit{and} \hspace{3pt}EX_{-}\big(X_{-}X_{-}^{*}\big)^{-\frac{1}{2}}= EX_{-}^{*}\bigg(\sum_{i=1}^{n} \frac{u_i u_{i}^{*}}{\sigma_{i}} \bigg)
\end{align}

\section{The smallest singular value}
% Furthermore, via an application of Cauchy-Schwarz, for all $k$:
% \begin{align}
%     & \label{eq:distjdrows} d^{2}_{k} \leq \sum_{i=1}^{N}\bigg|\sum_{t=1}^{i} \sum_{m=0}^{(i-t)\land (n-k)}\binom{i-t}{m} \lambda^{i-t-m} \big\langle  w_{t-1},e_{k+m}\big\rangle\bigg|^{2}
% \end{align}

% So the last row should not depend on other rows, indeed:
% \begin{align}
%     & \nonumber 1=\sum_{i=1}^{N} \bigg[ \sum_{t=1}^{i} \lambda^{(i-t)} \big \langle w_{t-1},e_{n}\big\rangle\bigg] \big \langle c_{n}, \hat{e}_{i} \big \rangle \\ & \nonumber d_{n}^{2}  \leq \sum_{i=1}^{N} \bigg|\sum_{t=1}^{i} \lambda^{i-t} \big \langle w_{t-1},e_{n} \big \rangle \bigg|^{2} 
% \end{align}
It turns out that distance estimates between a length $N$ random vector(that represents the scalar ARMA trajectory) and $N-n+1$ dimensional subspace as in subsection \ref{subsec:rowsubdist}, play a crucial role in dictating the least singular value of the data matrix and consequently provide an upper bound on the estimation error related to OLS for identification of LTI systems as in \eqref{eq:srkfill}. As we can take conjugate transpose and write least singular value of the data matrix as:
\begin{equation}
    \sigma_{n}(X_{-}):= \inf_{a \in S^{n-1}} \|X_{-}^{*}a\|_{2}
\end{equation}
Leveraging upon the Hilbertian structure(orthogonal projections/inner products), given any subspace $V \subset \mathbb{R}^{n}$, we have that:
\begin{equation}
    \|X_{-}^{*}a\|_{2}^{2}= \|P_{V}(X_{-}^{*}a)\|_{2}^{2} + \|P_{V^{\perp}}(X_{-}^{*}a)\|_{2}^{2} \geq \|P_{V^{\perp}}(X_{-}^{*}a)\|_{2}^{2}. 
\end{equation}
Therefore,
\begin{align}
    \big\|X_{-}^{*}a\big\|_{2} \geq |a_{i}|d(y_i,n_i), \hspace{5pt} \textit{for all} \hspace{3pt} i \in [n].
\end{align}
Now if $a \in S^{n-1}$, then there exists an $i \in [n]$ such that $|a_{i}| \geq \frac{1}{\sqrt{n}}$. Subsequently,
\begin{align}
    P\bigg( \inf_{a \in S^{n-1}} \|X_{-}^{*}a\| \leq \delta  \bigg) =P\bigg( \exists \hspace{3pt} a \in S^{n-1}: \hspace{2pt} \|X_{-}^{*}a\| \leq \delta  \bigg) \leq  P\bigg( \exists \hspace{3pt} j \in [n]: \hspace{2pt} \frac{d(y_j,n_j)}{\sqrt{n}} \leq \delta  \bigg)
\end{align}
\begin{itemize}
    \item when we have independent rows union bound is not terribly wasteful, so: 
    \begin{align}
        \mathbb{P}\big(\sigma_{n}(X_{-}) \leq \delta \big) \leq \sum_{j=1}^{n} \mathbb{P}\bigg(d(y_j,n_j)\leq  \delta \sqrt{n} \bigg)
    \end{align}
    Let $w_{j} \in S^{N-1}$ be orthogonal unit vector to subspace $n_j$(not necessarily unique), if the rows are independent then $w_{j}$ can be chosen independently of $y_{j}$. Therefore:
    \begin{equation}
        \langle w_{j},y_{j}\rangle =\langle w_{j},P_{n_{j}^{\perp}}y_{j}\rangle \leq \big\| P_{n_{j}^{\perp}}y_{j}\big\|=d(y_{j},n_{j}),
    \end{equation}
    where inequality follows from Cauchy-Schwarz. Consequently:
    \begin{equation}
        \mathbb{P}\bigg(d(y_j,n_j)\leq \delta\sqrt{n}\bigg) \leq \mathbb{P}\bigg(\langle w_{j},y_{j}\rangle\leq \delta\sqrt{n}\bigg), 
    \end{equation}
    where controlling the last term is commonly studied under the name of \emph{anti-concentration or small ball probability}.
    \item rows with strong correlation(S-w-SSC-s), then union bound will essentially conclude vacuous estimates so its' better to bound
    \begin{align}
        \mathbb{P}\big(\sigma_{n}(X_{-}) \leq \delta \big) \leq   \mathbb{P}\bigg(\min_{j \in [n]} d(y_j,n_j)\leq \delta \sqrt{n} \bigg)  
    \end{align}
\end{itemize}
\subsection{Decomposition of sphere based on compressibility}
Ideas and notation in this subsection heavily borrows from the work of \cite{rudelson2014recent}, \cite{rudelson2009smallest} and \cite{cook2016spectral}. For a better estimate of least singular value, one has to take infimum separatley over compressibe and incompressible elements of $n-$ dimensional unit sphere.
\begin{definition}
      We define the support of a vector $x \in \mathbb{R}^{n}$ as
    \begin{equation}
        supp(x):=[j \in [n]: \langle x,e_{j} \rangle \neq 0].
    \end{equation}
    For $J \subset [n]$, we define $S^{J}$ as set of unit vectors supported on $J$. Given $\epsilon>0$ and $V \subset \mathbb{R}^{n}$, set of vectors with in $\epsilon$ euclidean distance from $V$ are denoted by $V_{\epsilon}$. Compressible vectors with parameters $(\delta, \epsilon)$ are unit vectors which are within $\epsilon$ euclidean distance from some vector supported on at most $\delta n$ coordinates and mathematically defined as: 
    \begin{equation}
        Comp(\delta,\epsilon):=S^{n-1} \bigcap \bigcup_{J \in \binom{\delta n}{n}} \big(S^{J}\big)_{\epsilon}.
    \end{equation}
    and complementary set of incompressible vectors:
    \begin{equation}
        Incomp(\delta,\epsilon):=S^{n-1}\setminus Comp(\delta,\epsilon)
    \end{equation}
    \begin{lemma}
    For a square random matrix $M$ with i.i.d enteries 
    \begin{equation}
    \mathbb{P}\bigg(\inf_{u \in \textit{Incomp} (\delta,\epsilon)} \big\| Mu \big\| \leq \frac{t}{\sqrt{n}} \bigg) \leq \frac{1}{\delta n}  \sum_{i=1}^{n} \mathbb{P}\bigg(d(y_i,n_i)\bigg)  
    \end{equation}    
\end{lemma}
    \begin{lemma}
    Fix $\delta,\epsilon \in(0,1)$
    and let $v \in Incomp(\delta, \epsilon)$, there is a set $P^{+} \subset [n]$ with $|P^{+}|\geq \delta n$ and $|v_{j}| \geq \frac{\epsilon}{\sqrt{n}}$ for all $j \in P^{+}$. Moreover, for all $\lambda \geq 1$ there is a set $P \subset [n]$ with $|P| \geq (1-\frac{1}{\lambda^2}) \delta n$ such that for all $j \in P$
    \begin{equation}
    \frac{\epsilon}{\sqrt{n}} \leq |v_{j}| \leq \frac{\lambda}{\sqrt{\delta n}}        
    \end{equation}
    \end{lemma}
    \begin{proof}
        Take $P^{+}:=\{j:|v_{j}| \geq \frac{\epsilon}{\sqrt{n}}\}$, as $v$ is at least distance $\epsilon$ from any unit vector with support at most $\delta n$, so $1= \sum_{j \in ([n] \setminus P^{+})} |v_{j}|^2 + \sum_{j \in P^{+}} |v_{j}|^2 \geq \sum_{j \in ([n] \setminus P^{+})} |v_{j}|^2 + \frac{\epsilon^2}{n}|P^{+}|$ 
    \end{proof}
Let $0<\nu_{1}:=(1-\frac{1}{\lambda^2}) \delta, \hspace{2pt}\nu_{2}:=\epsilon <1$ and $\nu_{3}:=\frac{\lambda}{\sqrt{\delta}}>1$. It is imperative to notice that regardless of $x \in Incomp(\delta,\epsilon)$, $(\nu_1,\nu_2,\nu_3)$ are only dependent on $(\delta,\epsilon)$.
\end{definition}

Controlling the infimum over the incompressible vectors. Let $p:=\mathbb{P}\big(d(y_{k},n_{k})< \epsilon_1 \big)$. Then notice that under the assumption of independence between the rows,
\begin{equation}
    \mathbb{E} \big|\{k:d(y_k,n_k)< \epsilon \} \big|=\sum_{k=1}^{n} k\mathbb{P}\big(B=k\big)= \sum_{k=1}^{n}k \binom{n}{k} p^{k}(1-p)^{n-k}=np.   
\end{equation}
If we denote by $U$ the event that the cardinality of the set, $\sigma_{1}:=\{k:d(y_{k},n_{k}) \geq \epsilon_1\}$ contains more that $(1-\nu_{1})n$ elements. Then by Chebyshevs' inequality we have that:
\begin{equation}
    \mathbb{P}(U^c) \leq \frac{p}{\nu_{1}}
\end{equation}
and eventually:
\begin{equation}
    \mathbb{P}\bigg( \inf_{a \in Incomp(\delta,\epsilon)} \big\|X_{-}^{*}a \big\|< \frac{\epsilon_{1} \nu_{2}}{\sqrt{n}}\bigg) \leq \mathbb{P}(U^c) \leq \frac{\mathbb{P}\big(d(y_{k},n_{k})< \epsilon_1 \big)}{\nu_{1}}
\end{equation}
It is not too difficult to realize now, when dynamics are generated from Hermitian linear transformation, we can use concentration of measure to understand the behavior of least singular value.
\label{sec:concmdistsigma1}
Now we are left with the task of studying the typical order of $\|y_{n}\|^2$

Furthermore, 
$\lambda_{1}(\Sigma_{2}) \geq \underbrace{|\langle y_{n},y_{n} \rangle|}_{:= \lambda_{1}(\Sigma_{1})} \geq \lambda_{2}(\Sigma_{2})$. Now trivially, 
\begin{equation}
    \lambda_{1}(\Sigma_{2})= \max{\big(\sqrt{\langle y_{n-1},y_{n-1}\rangle^{2}+ \langle y_{n-1},y_{n}\rangle^{2}},  \sqrt{\langle y_{n},y_{n}\rangle^{2}+ \langle y_{n-1},y_{n}\rangle^{2}}  \big)}
\end{equation}
So in the case of S-w-SSCs, $ \lambda_{1}(\Sigma_{2})= \langle y_{n-1},y_{n-1}\rangle^{2}+ \langle y_{n-1},y_{n}\rangle^{2}$ and
\begin{equation}
\lambda_{2}(\Sigma_{2})= \inf_{a \in S^{1}} \sqrt{(a_{1} \langle y_{n-1},y_{n-1} \rangle+ a_{2}\langle y_{n},y_{n-1}\rangle)^2+ (a_{1} \langle y_{n-1},y_{n}\rangle+ a_{2}\langle y_{n},y_{n}\rangle)^2}= \inf_{a \in S^{1}} \|\Sigma_{2}a\|.    
\end{equation}
Assuming everything is real, computing  $\lambda_{2}^{2}(\Sigma_{2})$ would essentially require minimizing:
\begin{align}
    \nonumber & a_{1}^{2}\|y_{n-1}\|^2+a_{1}^{2}\langle y_{n-1},y_{n} \rangle^2+a_{2}^{2}\langle y_{n},y_{n-1} \rangle^2+ a_{2}^{2}\|y_n\|^2 +2a_{1}a_{2}\langle y_{n},y_{n-1} \rangle(\|y_{n-1}\|^{2}+\|y_n\|^{2}), 
\end{align}
over feasible $a_{1}, a_{2}$, i.e.,
\begin{align}
    \label{eq:cond1} & 2a_1\big(\|y_{n-1}\|^{2}+\langle y_{n-1},y_n\rangle^2\big)+2a_{2}\langle y_{n},y_{n-1}\rangle\big(\|y_{n-1}\|^{2}+\|y_n\|^{2}\big)=0 \\ \label{eq:cond2} & 2a_2\big(\|y_{n}\|^{2}+\langle y_{n-1},y_n\rangle^2\big)+2a_{1}\langle y_{n},y_{n-1}\rangle\big(\|y_{n-1}\|^{2}+\|y_n\|^{2}\big)=0  
\end{align}
Again using the preceding argument:
\begin{align}
    \nonumber  \lambda_{1}^{2}(\Sigma_3) = & \big(\|y_{n-2}\|^{2}+ \langle y_{n-2},y_{n-1}\rangle^{2}+\langle y_{n-2}, y_{n}\rangle^{2}\big) \vee \big(\langle y_{n-2},y_{n-1}\rangle^{2}+ \|y_{n-1}\|^{2}+\langle y_{n-1},y_{n}\rangle^{2}\big) \\ \nonumber & \vee  \big(\|y_n\|^{2}+ \langle y_{n-2} y_{n}\rangle^{2}+\langle y_{n-1},y_{n}\rangle^2\big)
\end{align}
For S-w-SSCs case: guess $\lambda_{1}(\Sigma_{3})=\sqrt{\langle y_{n-2},y_{n-2}\rangle^{2}+ \langle y_{n-2},y_{n-1}\rangle^{2}+\langle y_{n-2},y_{n}\rangle^{2}}$
\begin{equation}
    \lambda_{2}(\Sigma_{3})=\sup_{V_{2} \subset \mathbb{R}^{3}} \hspace{3pt} \inf_{a \in V_{2}\cap S^{2}} \|\Sigma_{3}a\|,
\end{equation}

\begin{align}
\nonumber &\lambda_{2}^{2}(\Sigma_{3})= \inf_{a \in S^{1}}\bigg[ (a_{1} \langle y_{n-2},y_{n-2} \rangle+ a_{2}\langle y_{n-2},y_{n-1}\rangle)^2+ (a_{1} \langle y_{n-1},y_{n-2}\rangle+ a_{2}\langle y_{n-1},y_{n-1}\rangle)^2 \\ \nonumber & \hspace{45pt} + (a_{1} \langle y_{n},y_{n-2}\rangle+ a_{2}\langle y_{n},y_{n-1}\rangle)^2\bigg]
\end{align}

% \begin{figure*}
% \label{fig:covmat}
% \begin{align*}
% \Sigma_{N,\lambda}:=
% \begin{pmatrix}
% 1 & \lambda & \lambda^2 & \lambda^3 & \ldots  \\
% \lambda & 1+\lambda^{2}  & \lambda^3+\lambda & \ldots & \ldots  \\
% \lambda^2 & \lambda^3+\lambda & 1+\lambda^2+\lambda^4 & \lambda^{5}+\lambda^{3}+\lambda &    \lambda^{N+1}+\lambda^{N-1}+ \lambda^{N-3}     \\
%  \ldots & \ldots & \ldots & \ldots\\
% \lambda^{N-1} &\lambda^{N}+\lambda^{N-1} & \ldots & \ldots &\ldots& \lambda^{2(N-1)}+\lambda^{2(N-2)}+ \ldots +1 \\    
% \end{pmatrix}
% \end{align*}
% \end{figure*}
% \begin{align}
%    \nonumber d^{2}(x,\mathcal{V}) &=\sum_{j=1}^{N}\bigg[(1-p_{jj})-2\sum_{k>j}^{N}a_{jk} \lambda^{[k-j]} \bigg]x_{j}^{2} \\ & \nonumber -2\sum_{j=1}^{N} x_{j}\sum_{k>j}^{N} a_{jk}\bigg[\lambda^{[k-j]-1}w_{j}+ \ldots +w_{k-1}\bigg].
% \end{align}
